# Supplementary material for: Direct measurement of a $\sin(2\varphi)$ current phase relation in a graphene superconducting quantum interference device
Source: arXiv:2405.13642 ancillary file (2024-05-22)
Supplement: Supplementary file 1 [file Messelot_graphene_doubleSQUID__SM.pdf]

**Supplemental Material for "Direct measurement of a  $\sin(2\varphi)$   
current phase relation in a graphene superconducting  
quantum interference device"**

## I. FABRICATION

We fabricated the hBN-graphene-hBN heterostructure using a dry transfer technique with Polypropylene carbonate (PPC) [1], from flakes exfoliated on Si/SiO<sub>2</sub> substrates. The heterostructure was subsequently released on a high resistivity intrinsic silicon substrate with pre-patterned alignment marks for subsequent e-beam lithography, by melting the PPC at 145°C after contacting the heterostructure onto the substrate. Melted PPC was washed away using an overnight acetone bath and remaining residues were eliminated by annealing the structure for 2 hours in a vacuum oven at 350°C. We defined the three junctions superconducting electrodes, both loops and all electrical connections using a first e-beam lithography step. After a cold development in an IPA-DI water 3:1 solution at 3°C for 90 s followed by 60 s rinse in water, we etched the top hBN, the graphene and part of the bottom hBN layer using CHF<sub>3</sub> based reactive ion etching (RIE). Immediately afterwards, we deposited 5/60 nm of Ti-Al using an e-beam evaporator to realize 1D contacts. Standard lift-off was next performed in acetone. We then removed excess graphene to define the junctions using a second e-beam lithography and a similar RIE process. The gate dielectric hBN layer was exfoliated on a Gelpack 4 polydimethylsiloxane (PDMS) stamp and released on top of the device by alignment and contact at 100°C followed by slow lift up of the stamp. PDMS residues were then removed using toluene at 80°C for 4 hours. Finally, we deposited the top gate electrodes with a third lithography step followed by 80 nm Al deposition and lift-off. The structure of the resulting Josephson junction structure is represented [Fig. S1](#).

The topmost hBN layer serves as gate dielectric between the junction contact electrodes and the top gate electrode, which enables capacitive control of the charge carrier density in the graphene weak link. Due to the 400 nm length of the junctions and the stiffness of hBN, there is a vacuum gap between the hBN gate dielectric and the hBN-graphene-hBN heterostructure. Away from the junction, the hBN gate dielectric adapts to the device profile during the deposition step. The 5 nm titanium layer of the contact electrodes ensures relative work function adaptation with graphene, preventing the formation of a strong Schottky barrier at the graphene-superconducting contact interface.

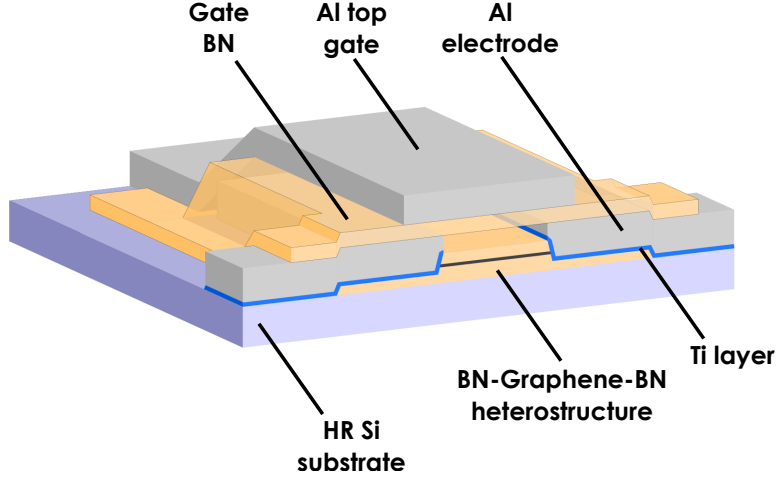

Figure S1. Structure of the Josephson junction, cut along the current axis, with the additional hBN gate dielectric and the top gate.

## II. EFFECT OF THE WIRE INDUCTANCE

We discuss the contribution of the reference branch inductance  $L_3$ , which is dominant since it is the longer wire, in which the largest current  $\simeq I_{c3}$  flows. Let us recall the approximate analytical expression of the full device positive and negative critical current:

$$I_c^\pm = \pm I_{c3} + I_2(\pm\varphi_{max} \pm 2\pi \frac{I_{c3}L_3}{\phi_0} + 2\pi \frac{\phi_2}{\phi_0}) + I_1(\pm\varphi_{max} \pm 2\pi \frac{I_{c3}L_3}{\phi_0} + 2\pi \frac{\phi_2}{\phi_0} + 2\pi \frac{\phi_1}{\phi_0}) \quad (1)$$

where we included the phase contribution of the current  $\pm I_{c3}$  flowing through  $L_3$  in addition to the expression given in the main text. The Josephson element CPR  $I_{JE}(\varphi) = I_2(\varphi) + I_1(\varphi + 2\pi \frac{\phi_1}{\phi_0})$  that we extract from our data is then X-shifted (i.e. along the current axis) in opposite directions depending on the current bias polarity. Note that  $\varphi_{max}$  has the same type of contribution to  $I^\pm$ , which accounts for the inversion of current sign in JJ<sub>3</sub>. Since the reference junction JJ<sub>3</sub> is an SNS junction,  $\varphi_{max} > \frac{\pi}{2}$  and the precise value is dependent on the transmission of JJ<sub>3</sub>. We cannot determine the latter independently from our measurement.

For these reasons, we cannot estimate unambiguously the value of  $L_3$  or  $\varphi_{max}$  from fit parameters because both parameters have the same contribution to the critical current

data. We observe a shift of  $\sim 0.7 \mu\text{T}$  (or  $0.9 \text{ rad}$ ) between  $I_c^+$  and  $I_c^-$ 's extrema positions versus magnetic field in the main text, see Fig. 2.a). Assuming a value of  $T_3 = 0.7$ , we find that  $L_3$  should amount to about  $30 \text{ pH}$  to take into account this shift. This value is in the range of the expected inductance for a  $60 \text{ nm}$ -thick aluminum line with  $50 \mu\text{m}$  length and  $1 \mu\text{m}$  width. With this assumption,  $\varphi_{max} > \frac{\pi}{2}$  is the principal cause of the offset, with an inductance  $L_3$  phase contribution limited to  $0.12 \text{ rad}$ .

### III. CRITICAL CURRENT VARIATIONS WITH THE GATE VOLTAGE.

We present critical current measurements using bias current sweeps as a function of the different top gate voltages. Figure S2 shows experimental data for  $\text{JJ}_1$ ,  $\text{JJ}_2$  and  $\text{JJ}_3$  while keeping other junctions closed, i.e. at their charge neutrality points. We find that the respective charge neutrality points are reached at  $V_{g1} = +1.4 \text{ V}$ ,  $V_{g2} = +3.0 \text{ V}$  and  $V_{g3} = -0.5 \text{ V}$ . The junctions showed hysteresis versus gate voltage limited typically to about  $300 \text{ mV}$ , after a first gate voltage sweep of  $\pm 6 \text{ V}$  for all junctions. The first sweeps, however, modified the charge neutrality point positions by up to  $+5 \text{ V}$ . This explains why measurements from the main text (see Fig. 1.c) are in the strongly n-doped regime, despite all gate voltages were initially kept at  $0 \text{ V}$ .

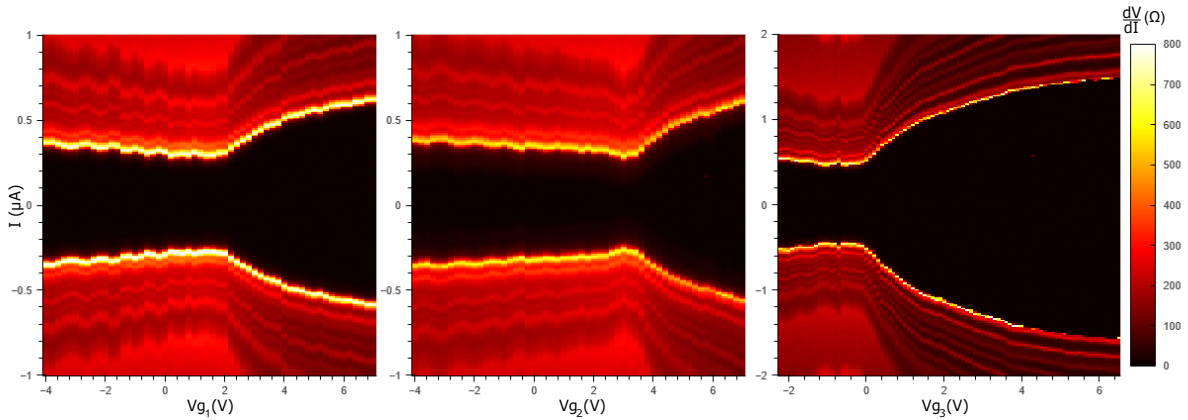

Figure S2. Differential resistance map of the double SQUID device versus bias current and top gate voltage for a)  $\text{JJ}_1$ , b)  $\text{JJ}_2$ , c)  $\text{JJ}_3$ , in the absence of magnetic field.

We observe the characteristic asymmetry between n- and p-doped regions for gate voltages lower or higher than the charge neutrality point respectively, indicating the formation of Schottky barriers at the aluminium-graphene interface in the p-doped regime.

Also, p-doped regions present critical current oscillations versus gate voltages characteristic of Fabry-Perot electronic interferences in the junction resulting in a modulation of the junction transparency [2].

#### IV. PHASE AND CURRENT ERRORS IN DC BIASED CPR MEASUREMENTS

The exact analytical expression of the critical current of the full Josephson element device is the maximum of the sum of all junctions currents:

$$I_c^+(\phi_1, \phi_2) = \max_{\varphi_{ref}} \left[ I_3(\varphi_{ref}) + I_{JE}(\varphi_{ref} + 2\pi \frac{\phi_2}{\phi_0}, \phi_1) \right] \quad (2)$$

The theoretical value of  $\Delta\varphi$  and  $I_3$  are then given [3, 4] by the solution of:

$$\frac{\partial I_3}{\partial \varphi_{ref}}(\varphi_{ref}) = -\frac{\partial I_{JE}}{\partial \varphi_{ref}}(\varphi_{ref} + 2\pi \frac{\phi_2}{\phi_0}) \quad (3)$$

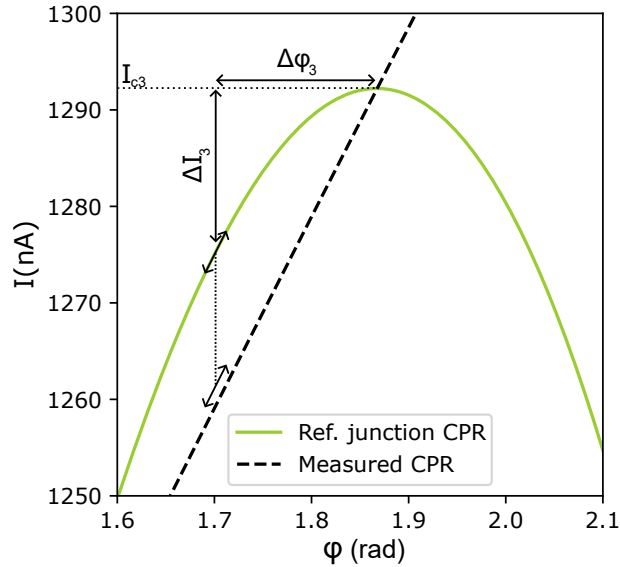

Figure S3. Graphical representation of the resolution of Eq. 3, showing  $I_3(\varphi)$  and  $-I_{JE}(\varphi + 2\pi \frac{\phi_2}{\phi_0})$  (vertically shifted,  $2\pi \frac{\phi_2}{\phi_0} = \frac{\pi}{2}$ ).

Figure S3.b) illustrates the graphical resolution of this equation: the CPR of the reference junction  $I_3(\varphi)$  (left side of the equation) is represented together with the opposite of the Josephson element CPR  $I_{JE}(\varphi + 2\pi\frac{\phi_2}{\phi_0})$  (right side of the equation). At the device critical current, both slopes matches as the maximum of the sum is reached. CPRs of SIS or SNS junctions are quadratic around their maxima with  $\frac{\partial I_3}{\partial \varphi_{ref}}(\varphi_{max}) = 0$ , and as a consequence,  $\varphi_{ref}$  always needs to deviate from  $\varphi_{max}$  to compensate for the investigated CPR derivative. This also results in a current drop in the reference junction  $\Delta I$ . Considering for clarity an SIS junction of critical current  $I_{c,ref}$ , simple expressions can be given:

$$\Delta\varphi \simeq -\frac{1}{I_{c,ref}} \frac{\partial I}{\partial \varphi} \quad , \quad \Delta I \simeq -\frac{1}{2I_{c,ref}} \left( \frac{\partial I}{\partial \varphi} \right)^2 \quad (4)$$

The respective linear and quadratic dependence of  $\Delta\varphi$  and  $\Delta I$  is apparent in Fig. 3.a) of the main text as the  $\sin(\varphi)$  term of the SQUID CPR grows linearly away from the frustration point. Eq. 4 demonstrates that the derivative of the investigated CPR is the relevant quantity regarding deviations of the reference phase. This is especially important for CPR with high harmonic content and large derivatives, for instance sawtooth-like CPR in long SNS junctions [5]. Also, since the phase deviation is linear versus  $\frac{\partial I}{\partial \varphi}$ , there is no general criterion for the appropriate ratio between critical currents of reference and investigated elements, and the phase and current errors are only inversely proportional to the reference junction critical current.

- 
- [1] L. Wang, I. Meric, P. Huang, Q. Gao, Y. Gao, H. Tran, T. Taniguchi, K. Watanabe, L. Campos, D. Muller, *et al.*, One-dimensional electrical contact to a two-dimensional material, *Science* **342**, 614 (2013).
  - [2] V. E. Calado, S. Goswami, G. Nanda, M. Diez, A. R. Akhmerov, K. Watanabe, T. Taniguchi, T. M. Klapwijk, and L. M. Vandersypen, Ballistic josephson junctions in edge-contacted graphene, *Nat. Nanotechnol.* **10**, 761 (2015).
  - [3] L. V. Ginzburg, I. Batov, V. V. Bol'ginov, S. V. Egorov, V. Chichkov, A. E. Shchegolev,

- N. V. Klenov, I. Soloviev, S. V. Bakurskiy, and M. Y. Kupriyanov, Determination of the current–phase relation in josephson junctions by means of an asymmetric two-junction SQUID, JETP Lett. **107**, 48 (2018).
- [4] I. Babich, A. Kudriashov, D. Baranov, and V. Stolyarov, Limitations of the current-phase relation measurements by an asymmetric dc-squid, arXiv:2302.02705 (2023).
- [5] J. Bardeen and J. L. Johnson, Josephson current flow in pure superconducting-normal-superconducting junctions, Phys. Rev. B **5**, 72 (1972).
